# Supplementary material for: Unified theoretical description of thermal and nonthermal laser-induced ultrafast structural changes in solids
Source: arXiv:2401.09922 ancillary file (2024-01-19)
Supplement: Supplementary file 1 [file supplemental_material.pdf]

# Supplemental Material
# Unified theoretical description of thermal and nonthermal laser-induced ultrafast structural changes in solids

Bernd Bauerhenne[1,2], Martin E. Garcia[1,2]

January 18, 2024

[1] Theoretical Physics, University of Kassel, Heinrich-Plett-Strasse 40, 34132 Kassel, Germany

[2] Center for Interdisciplinary Nanostructure Science and Technology (CINSaT), Heinrich-Plett-Strasse 40, 34132 Kassel, Germany

Correspondence to: bauerhen@uni-kassel.de

## Contents

**1 Implementation in the Velocity Verlet Algorithm S-2**
1.1 Remarks . . . . . . . . . . . . . . . . . . . . . . . . . . . . . . . S-9

**2 Direct comparison of the Bragg peak intensities with experiments S-11**
2.1 Electronic energy and specific heat of silicon . . . . . . . . . . S-11
2.2 Femtosecond-laser excitation below the damage threshold . . . S-12
2.3 Femtosecond-laser excitation above the damage threshold . . . S-16

# 1 Implementation in the Velocity Verlet Algorithm

We denote by $\vec{F}$ the vector containing all interatomic forces related to the potential energy surface

$$\vec{F} = -\nabla_{\vec{R}}\,\Phi \tag{S1}$$

and by $\vec{F}_{\text{tot}}$ the vector containing the total interatomic forces

$$\vec{F}_{\text{tot}} = \vec{F} + \sum_{k=1}^{N_{\mathcal{M}}} \xi_{\mathcal{M}_k}\, M\, \mathbf{P}_{\mathcal{M}_k} \cdot \vec{V}, \tag{S2}$$

$$\xi_{\mathcal{M}_k} = \frac{|\mathcal{M}_k|\, G_{\text{ep}_{\mathcal{M}_k}} \left(T_{\text{e}} - T_{\text{i}_{\mathcal{M}_k}}\right)}{2\, E_{\text{kin}_{\mathcal{M}_k}}}. \tag{S3}$$

In any MD simulation, we start from initial conditions $T_{\text{e}}(t_0)$, $\vec{R}(t_0)$, $\vec{V}(t_0)$, choose a time increment $\Delta t > 0$ and consider discrete times $t_\ell = t_0 + \ell\,\Delta t$, $\ell \in \mathbb{N}$, at which we want to calculate $T_{\text{e}}(t_\ell)$, $\vec{R}(t_\ell)$, $\vec{V}(t_\ell)$. For this, we have to integrate numerically the coupled differential equations of the ionic motions

$$M\,\frac{d\vec{V}}{dt} = \vec{F}_{\text{tot}}$$

and the differential equation for $T_{\text{e}}$

$$C_{\text{e}}\,\frac{dT_{\text{e}}}{dt} = \frac{dE_{\text{e}}}{dt}.$$

To integrate the ionic equations of motion, we choose the Velocity Verlet Algorithm, which calculates $\vec{R}$, $\vec{V}$, $\vec{F}$ at the next time step $t_\ell + \Delta t$ from the corresponding values of the previous time step $t_\ell$ via [5]

$$\vec{R}(t_{\ell+1}) = \vec{R}(t_\ell) + \Delta t\, \vec{V}(t_\ell) + \frac{\Delta t^2}{2\,M}\,\vec{F}_{\text{tot}}(t_\ell), \tag{S4}$$

$$\vec{V}(t_{\ell+1}) = \vec{V}(t_\ell) + \frac{\Delta t}{2\,M}\left(\vec{F}_{\text{tot}}(t_\ell) + \vec{F}_{\text{tot}}(t_{\ell+1})\right). \tag{S5}$$

Using $\vec{R}(t_0)$, we can calculate $\vec{F}(t_0)$, $\Phi(t_0)$, $S_{\text{e}}(t_0)$ and $C_{\text{e}}(t_0)$. We also know the phonon mode projection operators $P_{\mathcal{M}_k}$, which we assume to be time-independent. With the help of these projection operators $P_{\mathcal{M}_k}$ and $\vec{V}(t_0)$, we are able to calculate the kinetic energies $E_{\text{kin}_{\mathcal{M}_k}}(t_0)$, the temperatures $T_{\text{i}_{\mathcal{M}_k}}(t_0)$, and the terms $\xi_{\mathcal{M}_k}(t_0)$ of the different phonon mode sets

$\mathcal{M}_k$. Consequently, we are able to calculate the total force vector $\vec{F}_{\text{tot}}(t_0)$ at the starting time $t_0$ immediately from the initial conditions using Eq. (S2). From $\vec{R}(t_0)$, $\vec{V}(t_0)$ and $\vec{F}_{\text{tot}}(t_0)$, we are able to calculate $\vec{R}(t_1)$ from Eq. (S4).

However, now we cannot calculate directly $\vec{V}(t_1)$ from Eq. (S5), since we need for this $\vec{F}_{\text{tot}}(t_1)$, which can only be calculated from $\vec{V}(t_1)$ using Eq. (S2). If the electron-phonon coupling is neglected, $\vec{F}_{\text{tot}}(t_1)$ can be directly calculated from $\vec{R}(t_1)$ using $\Phi$ because of $\vec{F}_{\text{tot}}(t_1) = \vec{F}(t_1)$ and $\vec{V}(t_1)$ can be just calculated from Eq. (S5).

In the general case the electron-phonon coupling cannot be neglected, and we have to modify the procedure as follows: We consider a time step $t_\ell \geq t_0$ at which all quantities are known and want to calculate all quantities at time step $t_{\ell+1}$. At first, we calculate $\vec{R}(t_{\ell+1})$ from Eq. (S4). To derive $T_{\text{e}}(t_{\ell+1})$, we define further

$$\Delta E_{\text{L}_{\text{abs}}}(t_\ell) = \int\limits_{t_\ell}^{t_{\ell+1}} dt \, \frac{dE_{\text{L}_{\text{abs}}}(t)}{dt} = E_{\text{L}_{\text{abs}}}(t_{\ell+1}) - E_{\text{L}_{\text{abs}}}(t_\ell) \tag{S6}$$

as the energy that is absorbed by the electrons from the laser at time step $t_\ell$ and $\Delta E_{\text{ep}}(t_\ell)$ as the total energy that is transfered to the electrons from the ions due to electron-phonon coupling at time step $t_\ell$. We calculate numerically $\Delta E_{\text{ep}}(t_\ell)$ by

$$\Delta E_{\text{ep}}(t_\ell) = -\sum_{k=1}^{N_{\mathcal{M}}} |\mathcal{M}_k| \, G_{\text{ep}_{\mathcal{M}_k}}(t_\ell) \left( T_{\text{e}}(t_\ell) - T_{\text{i}_{\mathcal{M}_k}}(t_\ell) \right) \Delta t. \tag{S7}$$

From the total change of the electronic energy at time step $t_\ell$

$$\Delta E_{\text{e}}(t_\ell) = \Delta E_{\text{ep}}(t_\ell) + \Delta E_{\text{L}_{\text{abs}}}(t_\ell), \tag{S8}$$

we can calculate numerically the related change of $T_{\text{e}}$ for $C_{\text{e}}(t_\ell) > 0$ by

$$\Delta T_{\text{e}}(t_\ell) = \frac{\Delta E_{\text{e}}(t_\ell)}{C_{\text{e}}(t_\ell)} \overset{\text{(S8)}}{=} \frac{\Delta E_{\text{ep}}(t_\ell) + \Delta E_{\text{L}_{\text{abs}}}(t_\ell)}{C_{\text{e}}(t_\ell)}. \tag{S9}$$

From $\Delta T_{\text{e}}(t_\ell)$, we obtain $T_{\text{e}}(t_{\ell+1})$ just by

$$T_{\text{e}}(t_{\ell+1}) = T_{\text{e}}(t_\ell) + \Delta T_{\text{e}}(t_\ell). \tag{S10}$$

For $C_{\text{e}}(t_\ell) = 0$, we assume formally the ions as fixed and assign the change of the internal energy that is caused by varying $T_{\text{e}}$ to the electrons

$$\Delta E_{\text{e}}(t_\ell) = \Delta E(t_\ell)$$

$$=\Phi\left(T_{\mathrm{e}}(t_{\ell+1}),\vec{R}(t_\ell)\right)-T_{\mathrm{e}}(t_{\ell+1})\,\frac{d\Phi\left(T_{\mathrm{e}}(t_{\ell+1}),\vec{R}(t_\ell)\right)}{dT_{\mathrm{e}}}$$
$$-\Phi\Big(T_{\mathrm{e}}(t_\ell),\vec{R}(t_\ell)\Big)+T_{\mathrm{e}}(t_\ell)\,\frac{d\Phi\Big(T_{\mathrm{e}}(t_\ell),\vec{R}(t_\ell)\Big)}{dT_{\mathrm{e}}}. \tag{S11}$$

Now we solve numerically the equation above for $T_{\mathrm{e}}(t_{\ell+1})$. From $T_{\mathrm{e}}(t_{\ell+1})$ and $\vec{R}(t_{\ell+1})$, we can determine the quantities $\vec{F}(t_{\ell+1})$, $S_{\mathrm{e}}(t_{\ell+1})$ and $C_{\mathrm{e}}(t_{\ell+1})$. It is convenient to calculate also $G_{\mathrm{ep}_{\mathcal{M}_k}}(t_{\ell+1})$ at this point. In the most general case, we have

$$G_{\mathrm{ep}_{\mathcal{M}_k}}(t_{\ell+1})\equiv G_{\mathrm{ep}_{\mathcal{M}_k}}\left(T_{\mathrm{e}}(t_{\ell+1}),\vec{R}(t_{\ell+1}),\vec{V}(t_{\ell+1})\right).$$

Since $G_{\mathrm{ep}_{\mathcal{M}_k}}$ is a nontrivial function of $\vec{V}(t_{\ell+1})$ and we do not know $\vec{V}(t_{\ell+1})$ at this moment, we use $\vec{V}(t_\ell)$ to calculate $G_{\mathrm{ep}_{\mathcal{M}_k}}(t_{\ell+1})$:

$$G_{\mathrm{ep}_{\mathcal{M}_k}}(t_{\ell+1})\approx G_{\mathrm{ep}_{\mathcal{M}_k}}\left(T_{\mathrm{e}}(t_{\ell+1}),\vec{R}(t_{\ell+1}),\vec{V}(t_\ell)\right). \tag{S12}$$

Furthermore, we get for $\vec{V}(t_{\ell+1})$ by inserting Eq. (S2) for $\vec{F}_{\mathrm{tot}}(t_{\ell+1})$:

$$\vec{V}(t_{\ell+1})\overset{\text{(S5)}}{=}\vec{V}(t_\ell)+\frac{\Delta t}{2\,m}\left(\vec{F}_{\mathrm{tot}}(t_\ell)+\vec{F}_{\mathrm{tot}}(t_{\ell+1})\right)$$
$$\overset{\text{(S2)}}{=}\vec{V}(t_\ell)+\frac{\Delta t}{2\,m}\left(\vec{F}_{\mathrm{tot}}(t_\ell)+\vec{F}(t_{\ell+1})\right)+\frac{\Delta t}{2}\sum_{k=1}^{N_{\mathcal{M}}}\xi_{\mathcal{M}_k}(t_{\ell+1})\,\mathbf{P}_{\mathcal{M}_k}\cdot\vec{V}(t_{\ell+1}).$$

We define

$$\vec{W}(t_{\ell+1}):=\vec{V}(t_\ell)+\frac{\Delta t}{2\,m}\left(\vec{F}_{\mathrm{tot}}(t_\ell)+\vec{F}(t_{\ell+1})\right), \tag{S13}$$

which we can calculate, since $\vec{F}(t_{\ell+1})$ can be determined from the already known $\vec{R}(t_{\ell+1})$ and $T_{\mathrm{e}}(t_{\ell+1})$ using $\Phi$. $\vec{W}(t_{\ell+1})$ corresponds to the velocity vector at time $t_{\ell+1}$, if the influence of the electron-phonon coupling is neglected at the time step $t_{\ell+1}$. We obtain the following from the properties of the phonon mode projection operators

$$\vec{V}(t_{\ell+1})=\vec{W}(t_{\ell+1})+\frac{\Delta t}{2}\sum_{k=1}^{N_{\mathcal{M}}}\xi_{\mathcal{M}_k}(t_{\ell+1})\,\mathbf{P}_{\mathcal{M}_k}\cdot\vec{V}(t_{\ell+1}),$$
$$\Leftrightarrow\quad\underbrace{\sum_{k=1}^{N_{\mathcal{M}}}\mathbf{P}_{\mathcal{M}_k}}_{=1}\cdot\vec{V}(t_{\ell+1})=\underbrace{\sum_{k=1}^{N_{\mathcal{M}}}\mathbf{P}_{\mathcal{M}_k}}_{=1}\cdot\vec{W}(t_{\ell+1})+\frac{\Delta t}{2}\sum_{k=1}^{N_{\mathcal{M}}}\xi_{\mathcal{M}_k}(t_{\ell+1})\,\mathbf{P}_{\mathcal{M}_k}\cdot\vec{V}(t_{\ell+1}).$$

Multiplying on the left side by $\mathbf{P}_{\mathcal{M}_i}$, where $i$ is arbitrary from $\{1,\dots,N_{\mathcal{M}}\}$, yields

$$\begin{aligned} \mathbf{P}_{\mathcal{M}_i}\cdot\vec{V}(t_{\ell+1}) =& \mathbf{P}_{\mathcal{M}_i}\cdot\vec{W}(t_{\ell+1}) + \frac{\Delta t}{2}\,\xi_{\mathcal{M}_i}(t_{\ell+1})\,\mathbf{P}_{\mathcal{M}_i}\cdot\vec{V}(t_{\ell+1}), \\ \Leftrightarrow\quad \mathbf{P}_{\mathcal{M}_i}\cdot\vec{W}(t_{\ell+1}) =& \left(1-\frac{\Delta t}{2}\,\xi_{\mathcal{M}_i}(t_{\ell+1})\right)\mathbf{P}_{\mathcal{M}_i}\cdot\vec{V}(t_{\ell+1}). \end{aligned}$$

Since $i$ was chosen arbitrarily, the above equation is valid for all $i\in\{1,\dots,N_{\mathcal{M}}\}$. For a consistent notation, we change $i$ back to $k$ and obtain $\forall\ k\in\{1,\dots,N_{\mathcal{M}}\}$:

$$\mathbf{P}_{\mathcal{M}_k}\cdot\vec{V}(t_{\ell+1}) = \frac{1}{1-\frac{\Delta t}{2}\,\xi_{\mathcal{M}_k}(t_{\ell+1})}\,\mathbf{P}_{\mathcal{M}_k}\cdot\vec{W}(t_{\ell+1}). \tag{S14}$$

$\mathbf{P}_{\mathcal{M}_k}\cdot\vec{V}(t_{\ell+1})$ could be calculated from this equation if we knew $\xi_{\mathcal{M}_k}(t_{\ell+1})$, since we already determined $\vec{W}(t_{\ell+1})$. To derive $\xi_{\mathcal{M}_k}(t_{\ell+1})$, we consider the kinetic energy $E_{\mathrm{kin}_{\mathcal{M}_k}}(t_{\ell+1})$ of the phonon mode set $\mathcal{M}_k$:

$$\begin{aligned} E_{\mathrm{kin}_{\mathcal{M}_k}}(t_{\ell+1}) &= \frac{M}{2}\left(\mathbf{P}_{\mathcal{M}_k}\cdot\vec{V}(t_{\ell+1})\right)^{\mathrm{t}}\cdot\mathbf{P}_{\mathcal{M}_k}\cdot\vec{V}(t_{\ell+1}) \\ &\overset{(\mathrm{S14})}{=} \frac{1}{\left(1-\frac{\Delta t}{2}\,\xi_{\mathcal{M}_\ell}(t_{\ell+1})\right)^2}\,\frac{M}{2}\left(\mathbf{P}_{\mathcal{M}_k}\cdot\vec{W}(t_{\ell+1})\right)^{\mathrm{t}}\cdot\mathbf{P}_{\mathcal{M}_k}\cdot\vec{W}(t_{\ell+1}). \end{aligned}$$

We define

$$H_{\mathcal{M}_k}(t_{\ell+1}) := \frac{M}{2}\left(\mathbf{P}_{\mathcal{M}_k}\cdot\vec{W}(t_{\ell+1})\right)^{\mathrm{t}}\cdot\mathbf{P}_{\mathcal{M}_k}\cdot\vec{W}(t_{\ell+1}), \tag{S15}$$

which we can calculate directly from the determined $\vec{W}(t_{\ell+1})$. $H_{\mathcal{M}_k}(t_{\ell+1})$ corresponds to the kinetic energy of the phonon mode set $\mathcal{M}_k$ at time step $t_{\ell+1}$, if the influence of the electron-phonon coupling is neglected at the time step $t_{\ell+1}$. We get

$$E_{\mathrm{kin}_{\mathcal{M}_k}}(t_{\ell+1}) = \frac{H_{\mathcal{M}_k}(t_{\ell+1})}{1-\Delta t\,\xi_{\mathcal{M}_\ell}(t_{\ell+1})+\frac{\Delta t^2}{4}\,\xi_{\mathcal{M}_\ell}(t_{\ell+1})^2} \tag{S16}$$

and obtain for the parameter $\xi_{\mathcal{M}_k}$ at time step $t_{\ell+1}$:

$$\xi_{\mathcal{M}_k}(t_{\ell+1}) \overset{(\mathrm{S3})}{=} \frac{|\mathcal{M}_k|\,G_{\mathrm{ep}_{\mathcal{M}_k}}(t_{\ell+1})\left(T_{\mathrm{e}}(t_{\ell+1})-T_{\mathrm{i}_{\mathcal{M}_k}}(t_{\ell+1})\right)}{2\,E_{\mathrm{kin}_{\mathcal{M}_k}}(t_{\ell+1})}$$

$$
\begin{aligned}
&= \frac{|\mathcal{M}_k|\, G_{\mathrm{ep}_{\mathcal{M}_k}}(t_{\ell+1}) \left( T_\mathrm{e}(t_{\ell+1}) - \frac{2\, E_{\mathrm{kin}_{\mathcal{M}_k}}(t_{\ell+1})}{|\mathcal{M}_k|\, k_\mathrm{B}} \right)}{2\, E_{\mathrm{kin}_{\mathcal{M}_k}}(t_{\ell+1})} \\
&= \frac{|\mathcal{M}_k|\, G_{\mathrm{ep}_{\mathcal{M}_k}}(t_{\ell+1})\, T_\mathrm{e}(t_{\ell+1})}{2\, E_{\mathrm{kin}_{\mathcal{M}_k}}(t_{\ell+1})} - \frac{G_{\mathrm{ep}_{\mathcal{M}_k}}(t_{\ell+1})}{k_\mathrm{B}} \\
&\overset{(\mathrm{S16})}{=} \frac{|\mathcal{M}_k|\, G_{\mathrm{ep}_{\mathcal{M}_k}}(t_{\ell+1})\, T_\mathrm{e}(t_{\ell+1})}{2\, H_{\mathcal{M}_k}(t_{\ell+1})} \left( 1 - \Delta t\, \xi_{\mathcal{M}_\ell}(t_{\ell+1}) + \frac{\Delta t^2}{4}\, \xi_{\mathcal{M}_\ell}(t_{\ell+1})^2 \right) \\
&\quad - \frac{G_{\mathrm{ep}_{\mathcal{M}_k}}(t_{\ell+1})}{k_\mathrm{B}}. \qquad \text{(S17)}
\end{aligned}
$$

Since all quantities are considered at time step $t_{\ell+1}$, we omit the time argument $(t_{\ell+1})$ in the following for brevity. Now we solve this quadratic equation for $\xi_{\mathcal{M}_k}$:

$$
\begin{aligned}
0 =& \frac{|\mathcal{M}_k|\, G_{\mathrm{ep}_{\mathcal{M}_k}}\, T_\mathrm{e}\, \Delta t^2}{8\, H_{\mathcal{M}_k}}\, \xi_{\mathcal{M}_k}^2 - \left( 1 + \frac{|\mathcal{M}_k|\, G_{\mathrm{ep}_{\mathcal{M}_k}}\, T_\mathrm{e}\, \Delta t}{2\, H_{\mathcal{M}_k}} \right) \xi_{\mathcal{M}_k} \\
&+ \frac{|\mathcal{M}_k|\, G_{\mathrm{ep}_{\mathcal{M}_k}}\, T_\mathrm{e}}{2\, H_{\mathcal{M}_k}} - \frac{G_{\mathrm{ep}_{\mathcal{M}_k}}}{k_\mathrm{B}}, \\
\Leftrightarrow \qquad 0 =& \xi_{\mathcal{M}_k}^2 - \left( \frac{8\, H_{\mathcal{M}_k}}{|\mathcal{M}_k|\, G_{\mathrm{ep}_{\mathcal{M}_k}}\, T_\mathrm{e}\, \Delta t^2} + \frac{4}{\Delta t} \right) \xi_{\mathcal{M}_k} + \frac{4}{\Delta t^2} \\
&- \frac{8\, H_{\mathcal{M}_k}}{k_\mathrm{B}\, |\mathcal{M}_k|\, G_{\mathrm{ep}_{\mathcal{M}_k}}\, T_\mathrm{e}\, \Delta t^2}, \\
\Rightarrow \quad \xi_{\mathcal{M}_k} =& \frac{4\, H_{\mathcal{M}_k}}{|\mathcal{M}_k|\, G_{\mathrm{ep}_{\mathcal{M}_k}}\, T_\mathrm{e}\, \Delta t^2} + \frac{2}{\Delta t} \\
&- \sqrt{ \left( \frac{4\, H_{\mathcal{M}_k}}{|\mathcal{M}_k|\, G_{\mathrm{ep}_{\mathcal{M}_k}}\, T_\mathrm{e}\, \Delta t^2} + \frac{2}{\Delta t} \right)^2 + \frac{8\, H_{\mathcal{M}_k}}{k_\mathrm{B}\, |\mathcal{M}_k|\, G_{\mathrm{ep}_{\mathcal{M}_k}}\, T_\mathrm{e}\, \Delta t^2} - \frac{4}{\Delta t^2} }. \\
& \qquad \text{(S18)}
\end{aligned}
$$

$\xi_{\mathcal{M}_k}$ increases or decreases the velocity of ions in the direction of the velocities of the phonon modes from set $\mathcal{M}_k$. Since the velocities enter the kinetic energy quadratically, the sign of the velocity is not relevant for the energy conservation. Hence, there are two mathematical solutions for $\xi_{\mathcal{M}_k}$. The first solution changes the velocity slightly and thus corresponds to a small $\xi_{\mathcal{M}_k}$. That is the solution of Eq. (S18). The second solution changes the sign of the velocity or changes the direction of movement and thus corresponds to a large absolute value of $\xi_{\mathcal{M}_k}$. This unphysical solution is given by the "+" solution of the quadratic equation. To see that the "+" solution is one with

bigger magnitude, we let $a$ be the first two summands and $b$ be the square root in Eq. (S18), *i.e.*, $\xi_{\mathcal{M}_k} \overset{\text{(S18)}}{=} a \pm b$. We obtain $a \geq 0$ by construction and $b \geq 0$, if the square root has a real solution. We get finally from the triangle inequality: $|a - b| \leq |a| + |b| = a + b = |a + b|$.

Eq. (S18) is not valid for $G_{\text{ep}_{\mathcal{M}_k}} = 0$. In this case, we obtain $\xi_{\mathcal{M}_k} = 0$ from the definition of $\xi_{\mathcal{M}_k}$ in Eq. (S3). Eq. (S18) is also not valid for $T_\text{e} = 0$. Here, we get $\xi_{\mathcal{M}_k} = -\frac{G_{\text{ep}_{\mathcal{M}_k}}}{k_\text{B}}$ from Eq. (S17).

To calculate $E(t_{\ell+1})$, we define

$$I(t_\ell) := \int_{t_0}^{t_\ell} dt\, (S_\text{e} + C_\text{e})\, \frac{dT_\text{e}}{dt}. \tag{S19}$$

Thus, we get $I(t_0) = 0$ and $U(t_{\ell+1}) = \Phi(t_{\ell+1}) + I(t_{\ell+1})$. To calculate numerically $I(t_{\ell+1})$, we use $I(t_\ell)$ and approximate the remaining integral from $t_\ell$ to $t_{\ell+1}$ in (S19) by using the trapezoidal rule:

$$I(t_{\ell+1}) = I(t_\ell) + \frac{1}{2}\Big(\big(S_\text{e}(t_\ell) + C_\text{e}(t_\ell)\big)\,\Delta T_\text{e}(t_\ell) + \big(S_\text{e}(t_{\ell+1}) + C_\text{e}(t_{\ell+1})\big)\,\Delta T_\text{e}(t_{\ell+1})\Big). \tag{S20}$$

Now we have calculated all quantities at time step $t_{\ell+1}$ and summarize the calculation procedure:

$$\begin{aligned}
\vec{R}(t_{\ell+1}) &\overset{\text{(S4)}}{=} \vec{R}(t_\ell) + \Delta t\, \vec{V}(t_\ell) + \frac{\Delta t^2}{2\,m}\, \vec{F}_\text{tot}(t_\ell),\\
\Delta E_{\text{L}_\text{abs}}(t_\ell) &\overset{\text{(S6)}}{=} E_{\text{L}_\text{abs}}(t_{\ell+1}) - E_{\text{L}_\text{abs}}(t_\ell),\\
\Delta E_\text{ep}(t_\ell) &\overset{\text{(S7)}}{=} -\sum_{k=1}^{N_\mathcal{M}} |\mathcal{M}_k|\, G_{\text{ep}_{\mathcal{M}_k}}(t_\ell)\,\Big(T_\text{e}(t_\ell) - T_{\text{i}_{\mathcal{M}_k}}(t_\ell)\Big)\,\Delta t,\\
\Delta T_\text{e}(t_\ell) &\overset{\text{(S9)}}{=} \frac{\Delta E_\text{ep}(t_\ell) + \Delta E_{\text{L}_\text{abs}}(t_\ell)}{C_\text{e}(t_\ell)},\\
T_\text{e}(t_{\ell+1}) &\overset{\text{(S10)}}{=} T_\text{e}(t_\ell) + \Delta T_\text{e}(t_\ell),\\
S_\text{e}(t_{\ell+1}) &= -\frac{\partial \Phi\Big(T_\text{e}(t_{\ell+1}), \vec{R}(t_{\ell+1})\Big)}{\partial T_\text{e}},\\
C_\text{e}(t_{\ell+1}) &= -T_\text{e}(t_{\ell+1})\, \frac{\partial^2 \Phi\Big(T_\text{e}(t_{\ell+1}), \vec{R}(t_{\ell+1})\Big)}{\partial T_\text{e}^2},
\end{aligned}$$

$$
\begin{aligned}
\vec{F}(t_{\ell+1}) &\overset{\text{(S1)}}{=} \begin{bmatrix} -\nabla_{\mathbf{r}_1}\Phi\Big(T_\mathrm{e}(t_{\ell+1}),\vec{R}(t_{\ell+1})\Big) \\ \vdots \\ -\nabla_{\mathbf{r}_{N_\mathrm{at}}}\Phi\Big(T_\mathrm{e}(t_{\ell+1}),\vec{R}(t_{\ell+1})\Big) \end{bmatrix}, \\
G_{\mathrm{ep}_{\mathcal{M}_k}}(t_{\ell+1}) &\overset{\text{(S12)}}{=} G_{\mathrm{ep}_{\mathcal{M}_k}}\Big(T_\mathrm{e}(t_{\ell+1}),\vec{R}(t_{\ell+1}),\vec{V}(t_\ell)\Big), \\
\vec{W}(t_{\ell+1}) &\overset{\text{(S13)}}{=} \vec{V}(t_\ell) + \frac{\Delta t}{2\,M}\Big(\vec{F}_\mathrm{tot}(t_\ell) + \vec{F}(t_{\ell+1})\Big), \\
H_{\mathcal{M}_k}(t_{\ell+1}) &\overset{\text{(S15)}}{=} \frac{M}{2}\Big(\mathbf{P}_{\mathcal{M}_k}\cdot\vec{W}(t_{\ell+1})\Big)^\mathrm{t}\cdot\mathbf{P}_{\mathcal{M}_k}\cdot\vec{W}(t_{\ell+1}), \\
\xi_{\mathcal{M}_k}(t_{\ell+1}) &\overset{\text{(S18)}}{=} \frac{4\,H_{\mathcal{M}_k}(t_{\ell+1})}{|\mathcal{M}_k|\,G_{\mathrm{ep}_{\mathcal{M}_k}}(t_{\ell+1})\,T_\mathrm{e}(t_{\ell+1})\,\Delta t^2} + \frac{2}{\Delta t} \\
&\quad - \sqrt{\begin{aligned}&\left(\frac{4\,H_{\mathcal{M}_k}(t_{\ell+1})}{|\mathcal{M}_k|\,G_{\mathrm{ep}_{\mathcal{M}_k}}(t_{\ell+1})\,T_\mathrm{e}(t_{\ell+1})\,\Delta t^2} + \frac{2}{\Delta t}\right)^2 \\ &+ \frac{8\,H_{\mathcal{M}_k}(t_{\ell+1})}{k_\mathrm{B}\,|\mathcal{M}_k|\,G_{\mathrm{ep}_{\mathcal{M}_k}}\,T_\mathrm{e}(t_{\ell+1})\,\Delta t^2} - \frac{4}{\Delta t^2}\end{aligned}}, \\
\vec{V}(t_{\ell+1}) &\overset{\text{(S14)}}{=} \sum_{k=1}^{N_\mathcal{M}} \frac{1}{1-\frac{\Delta t}{2}\,\xi_{\mathcal{M}_k}(t_{\ell+1})}\,\mathbf{P}_{\mathcal{M}_k}\cdot\vec{W}(t_{\ell+1}). \\
\vec{F}_\mathrm{tot}(t_{\ell+1}) &\overset{\text{(S2)}}{=} \vec{F}(t_{\ell+1}) + \sum_{k=1}^{N_\mathcal{M}} \xi_{\mathcal{M}_k}(t_{\ell+1})\,M\,\mathbf{P}_{\mathcal{M}_k}\cdot\vec{V}(t_{\ell+1}), \\
E_{\mathrm{kin}_{\mathcal{M}_k}}(t_{\ell+1}) &\overset{\text{(S2)}}{=} \frac{M}{2}\,\vec{V}(t_{\ell+1})^\mathrm{t}\cdot\mathbf{P}_{\mathcal{M}_k}\cdot\vec{V}(t_{\ell+1}), \\
T_{\mathrm{i}_{\mathcal{M}_k}}(t_{\ell+1}) &= \frac{2\,E_{\mathrm{kin}_{\mathcal{M}_k}}(t_{\ell+1})}{|\mathcal{M}_k|\,k_\mathrm{B}}, \\
\Delta E_{\mathrm{L_{abs}}}(t_{\ell+1}) &\overset{\text{(S6)}}{=} E_{\mathrm{L_{abs}}}(t_{\ell+2}) - E_{\mathrm{L_{abs}}}(t_{\ell+1}), \\
\Delta E_\mathrm{ep}(t_{\ell+1}) &\overset{\text{(S7)}}{=} -\sum_{k=1}^{N_\mathcal{M}} |\mathcal{M}_k|\,G_{\mathrm{ep}_{\mathcal{M}_k}}(t_{\ell+1})\Big(T_\mathrm{e}(t_{\ell+1}) - T_{\mathrm{i}_{\mathcal{M}_k}}(t_{\ell+1})\Big)\,\Delta t, \\
\Delta T_\mathrm{e}(t_{\ell+1}) &\overset{\text{(S9)}}{=} \frac{\Delta E_\mathrm{ep}(t_{\ell+1}) + \Delta E_{\mathrm{L_{abs}}}(t_{\ell+1})}{C_\mathrm{e}(t_{\ell+1})}, \\
I(t_{\ell+1}) &\overset{\text{(S20)}}{=} I(t_\ell) \\
&\quad + \frac{1}{2}\Big(\big(S_\mathrm{e}(t_\ell) + C_\mathrm{e}(t_\ell)\big)\,\Delta T_\mathrm{e}(t_\ell) \\
&\qquad + \big(S_\mathrm{e}(t_{\ell+1}) + C_\mathrm{e}(t_{\ell+1})\big)\,\Delta T_\mathrm{e}(t_{\ell+1})\Big),
\end{aligned}
$$

$$E(t_{\ell+1}) \;=\; \Phi\Big(T_{\mathrm{e}}(t_{\ell+1}), \vec{R}(t_{\ell+1})\Big) + I(t+\Delta t).$$

If the above algorithm is implemented, every quantity only needs to be stored at the actual time step $t_{\ell+1}$ and the previous time step $t_\ell$.

## 1.1 Remarks

- As already mentioned, our modeling of the electron-phonon coupling can also be implemented in $T_{\mathrm{e}}$-dependent DFT, so that $\Phi$ corresponds to the Helmholtz free energy $F$ of the electrons.

- If no energy is absorbed from the laser field, *i.e.*, $E_{\mathrm{L_{abs}}} \equiv 0$, and the electron-phonon coupling is neglected, *i.e.*, $G_{\mathrm{ep}_{\mathcal{M}_k}} = 0$ for all $k \in \{1, \ldots, N_{\mathcal{M}}\}$, the electronic temperature $T_{\mathrm{e}}$ keeps constant. Then, the potential energy $E(t_\ell)$ of the ions and the electrons at $T_{\mathrm{e}}$ reduces to $\Phi(t_\ell)$, the energy conservation becomes $\Phi + E_{\mathrm{kin}} = \mathrm{const.}$ and the equation of motion for the ions reduces to $M\,\frac{d\vec{V}}{dt} = \vec{F}$. This corresponds just to the MD simulation setup commonly used in $T_{\mathrm{e}}$-dependent DFT.

- This modeling predicts perfect conservation of energy. Hence, the presented numerical implementation in the Velocity Verlet algorithm must not show any drift or fluctuation of the total energy $E + E_{\mathrm{kin}} - E_{\mathrm{L_{abs}}}$ during time propagation in the limit of $\Delta t \to 0$. This feature can be used to check the numerical implementation of the algorithm in the program.

- If a phonon mode set $\mathcal{M}_k$ contains only a small number of different modes, the corresponding ionic temperature $T_{\mathrm{i}_{\mathcal{M}_k}}$ will show significant fluctuations in time. Especially, if the set just contains one single phonon mode, the corresponding ionic temperature may be ill defined due to this fluctuations. Hence, every phonon mode set $\mathcal{M}_k$ should contain enough modes.

- If the lattice melts due to the laser excitation, the symmetry of the structure breaks. Therefore, in such cases, the consideration of different electron-phonon coupling constants $G_{\mathrm{ep}_{\mathcal{M}_k}}$ for specific phonon mode sets $\mathcal{M}_k$ may be non-physical, so that only one coupling constant should be used instead.

- Laser pulses with a Gaussian-shaped time profile are commonly used in experiments. Such pulses are characterized by the FWHM (full width at half maximum) time width $\tau$. Let $E_{\mathrm{L_{tot}}}$ be the total laser-absorbed

energy of the pulse. Then the total laser-absorbed energy rate at time $t_\ell$ is given by

$$\frac{dE_{\mathrm{L_{abs}}}(t_\ell)}{dt} = \frac{E_{\mathrm{L_{tot}}}}{\tau}\sqrt{\frac{\log(16)}{\pi}}\,\exp\left(-\frac{(t_\ell - 2\,\tau)^2}{\tau^2}\,\log(16)\right). \tag{S21}$$

Here, the MD simulation starts at $t_0 = 0$ and the maximal energy absorption rate is reached at time $2\,\tau$. 99.99975% of $E_{\mathrm{L_{tot}}}$ is absorbed during $t = 0$ and $t = 4\,\tau$. Using the Gauss error function

$$\mathrm{erf}(x) = \frac{2}{\sqrt{\pi}}\int_0^x dt\,^{-t^2} \tag{S22}$$

The total laser-absorbed energy up to time $t_\ell$ can be analytically calculated by:

$$\begin{aligned} E_{\mathrm{L_{abs}}}(t_\ell) &= \int_0^{t_\ell} dt\,\frac{dE_{\mathrm{L_{abs}}}(t)}{dt} \\ &= \frac{E_{\mathrm{L_{tot}}}}{2}\left(\mathrm{erf}\left(\sqrt{\log(65536)}\right) + \mathrm{erf}\left(\frac{t_\ell - 2\,\tau}{\tau}\,\sqrt{\log(16)}\right)\right). \end{aligned} \tag{S23}$$

Analogously, the total laser-absorbed energy at time step $t_\ell$ is calculated by

$$\begin{aligned} \Delta E_{\mathrm{L_{abs}}}(t_\ell) &= \int_{t_\ell}^{t_{\ell+1}} dt\,\frac{dE_{\mathrm{L_{abs}}}(t)}{dt} \\ &= \frac{E_{\mathrm{L_{tot}}}}{2}\left(-\mathrm{erf}\left(\frac{t_\ell - 2\,\tau}{\tau}\,\sqrt{\log(16)}\right)\right. \\ &\qquad \left. + \,\mathrm{erf}\left(\frac{t_{\ell+1} - 2\,\tau}{\tau}\,\sqrt{\log(16)}\right)\right). \end{aligned} \tag{S24}$$

- If a $T_\mathrm{e}$-dependent interatomic potential $\Phi$ is used in the MD simulation, $\Phi$ must exhibit a physical specific electronic heat

  $$C_\mathrm{e} = -T_\mathrm{e}\,\frac{\partial^2\Phi}{\partial T_\mathrm{e}^2}.$$

  The minimal requirement for a meaningful MD simulation is $C_\mathrm{e} \geq 0$.

- If one uses a $T_\mathrm{e}$-dependent interatomic potential in the MD simulation, the force $-\nabla_{\mathbf{r}_i}\Phi$ on any atom $i$ can be calculated only from the knowledge of the positions of the neighbors $j$ of atom $i$ within the cutoff radius $r^{(\mathrm{c})}$ of $\Phi$. This is used to parallelize MD simulations with an interatomic potential by separating the simulation cell in small sub cells, which can be treated independently of each other except for a small information exchange between neighboring cells. Using this parallelization, MD simulations of hundreds of millions of atoms are possible in a reasonable time. This parallelization may be impossible, if the projection on the phonon mode sets $\mathcal{M}_k$ is used to describe the electron-phonon coupling: In any phonon mode, all atoms of the structure show a collective motion. Hence, to calculate any component of

$$\vec{F}_\mathrm{tot} = \vec{F} + \sum_{k=1}^{N_\mathcal{M}} \xi_{\mathcal{M}_k}\, m\, \mathbf{P}_{\mathcal{M}_k} \cdot \vec{V},$$

we need always the knowledge of all atomic velocities. The total force on any atom $i$ can only be calculated, if the velocities of all other atoms are known to perform the necessary projection $\mathbf{P}_{\mathcal{M}_k} \cdot \vec{V}$. One solution to this problem may be a local definition of the projection operators $\mathbf{P}_{\mathcal{M}_k}$. The projection on the different phonon modes should only take explicitly the movement of neighboring atoms into account to be able to perform the common parallelization for speeding up.

# 2 Direct comparison of the Bragg peak intensities with experiments

## 2.1 Electronic energy and specific heat of silicon

In order to simulate only the EPC, we needed the electronic specific heat $C_\mathrm{e}(T_\mathrm{e})$ and the electronic internal energy $E_\mathrm{e}(T_\mathrm{e})$ as a function of $T_\mathrm{e}$. We considered the ideal diamond-like structure of Si with the optimal lattice parameter $a = 0.539872$ nm and derived the Helmholtz free energy $F(T_\mathrm{e})$ from $T_\mathrm{e}$-dependent DFT using CHIVES for various $T_\mathrm{e}$'s. We fitted $F(T_\mathrm{e})$ as a polynomial of degree 11 in $T_\mathrm{e}$ and derived $C_\mathrm{e}(T_\mathrm{e})$ from this polynomial using the thermodynamic relation $C_\mathrm{e} = -T_\mathrm{e}\,\frac{\partial^2 F}{\partial T_\mathrm{e}^2}$:

$$C_\mathrm{e}(T_\mathrm{e}) = N_\mathrm{at} \sum_{k=1}^{10} a_{C_\mathrm{e}}^{(k)} \left(\frac{T_\mathrm{e}}{31577\,\mathrm{K}}\right)^k . \tag{S25}$$

The coefficients $a_{C_e}^{(k)}$ are tabulated in Tab. S1. Since we are using a global $T_e$, we obtain the total electronic internal energy just by

$$E_e(T_e) = \int_0^{T_e} dT'_e \, C_e(T'_e). \tag{S26}$$

Tab. S1: Parametrization of the electronic specific heat $C_e(T_e)$ using Eq. (S25). The unit of $a_{C_e}^{(k)}$ is $\frac{\text{eV}}{\text{K atom}}$.

| $k$ | $a_{C_e}^{(k)}$ | $k$ | $a_{C_e}^{(k)}$ | $k$ | $a_{C_e}^{(k)}$ |
|---|---|---|---|---|---|
| 1 | 9.990955456836453E-6 | 2 | -6.188280768791413E-4 | 3 | 0.040068462158504514 |
| 4 | -0.26312331638621433 | 5 | 0.8576043019886007 | 6 | -1.679202915977002 |
| 7 | 2.069435128552068 | 8 | -1.5768394499029128 | 9 | 0.6799728970274491 |
| 10 | -0.12703240946979374 | | | | |

## 2.2 Femtosecond-laser excitation below the damage threshold

Harb *et al.* prepared a free standing polycrystalline Si film with a thickness of $d_{\text{film}} = 50$ nm [2]. They excited this film by an intense femtosecond laser-pulse with a central wavelength of $\lambda = 387$ nm and a FWHM-time width of $\tau = 150$ fs. The fluence of $I_{\text{L}_{\text{tot}}} = 5.6\,\frac{\text{mJ}}{\text{cm}^2}$ was absorbed at the surface, which is below the damage threshold of $I_{\text{L}_{\text{tot}}}^{(\text{damage})} = 6.5\,\frac{\text{mJ}}{\text{cm}^2}$. They measured the time-dependent intensity of serveral Bragg peaks using ultrafast electron diffraction.

To compare directly with this measurement, we set up a simulation cell that consists of $11 \times 11 \times 93$ conventional cells and contains $N_{\text{at}} = 90024$ Si atoms. We applied periodic boundary conditions in $x$- and $y$-direction and open boundary conditions in $z$-direction to get a 50 nm thick Si film. We used the Andersen thermostat [1] to initialize the atomic coordinates and velocities at $T_i = 300$ K.

Then we performed MD simulations of the femtosecond-laser excitation using the three different in the paper described scenarios – excited PES & EPC, only excited PES, only EPC. We used a time step of $\Delta t = 1$ fs and simulated a Gaußian-shaped pulse with a FWHM-time width of $\tau = 150$ fs similar to the experiment. To obtain the energy $E_{\text{L}_{\text{tot}}}$ absorbed from the laser from the measured absorbed fluence $I_{\text{L}_{\text{tot}}}$ at the surface, we have to consider the optical properties of Si. Harb *et al.* excited the Si film

with a femtosecond-laser having a central wavelength of $\lambda = 387$ nm, which corresponds to a photon energy of

$$E_{\text{phot}} = \frac{2\pi\,\hbar}{\lambda} = 3.2\,\text{eV}, \tag{S27}$$

where $\hbar$ denotes the reduced Planck's constant and  the speed of light in vacuum. At this photon energy, we found $n = 6.062 + 0.630\,i$ for the index of refraction of Si in literature [4]. Using this index of refraction, we obtained the absorption coefficient of Si of

$$\alpha_{\text{abs}} = \frac{4\pi}{\lambda}\,\text{Im}(n) = 0.0204569\,\frac{1}{\text{nm}}, \tag{S28}$$

where Im($n$) denotes the imaginary part of the index of refraction $n$. Using the ab-initio equilibrium atomic density $\rho_{\text{at}} = 50.8414\,\frac{\text{atoms}}{\text{nm}^3}$ and the experimental absorbed laser fluence $I_{\text{L}_{\text{tot}}} = 5.6\,\frac{\text{mJ}}{\text{cm}^2} = 349.525\,\frac{\text{eV}}{\text{nm}^2}$ at the surface, we obtained for the from the laser absorbed energy $E_{\text{L}_{\text{tot}}}$ in the 50 nm thick film

$$\frac{E_{\text{Ltot}}}{N_{\text{at}}} = \left(1 - {}^{-\alpha_{\text{abs}}\,d_{\text{film}}}\right)\frac{I_{\text{Ltot}}}{d_{\text{film}}\,\rho_{\text{at}}} \approx 0.1\,\frac{\text{eV}}{\text{atom}}, \tag{S29}$$

which we utilized in our MD simulations.

From the atomic coordinates, we derived the time-dependent intensities of the experimental studied Bragg peaks. In order to be able to compare directly with the experiments, we took into account, that Harb *et al.* did not measure the intensity of a single Bragg peak. Since they utilized a polycrystalline Si film, they obtained rings in the diffraction image instead of spots, which would be present for a monocrystalline film. They averaged the intensities within a ring of a given radius and labeled the resulting value by a Bragg peak, which diffraction peak is located inside the ring. Therefore, to derive the intensity of such a measured Bragg peak ($hkl$), we have to average the intensity over every Bragg peak with scattering vector $\mathbf{q}$ fulfilling the condition $|\mathbf{q}| \in \left[|\mathbf{G}_{hkl}| - \Delta q, |\mathbf{G}_{hkl}| + \Delta q\right]$. We chose here the broadening $\Delta q = 0.37\,\frac{1}{\text{nm}}$, so that the calculated relative Bragg peak intensity matches as good as possible to the measured one. We show, as an example, the influence of the broadening $\Delta q$ on the relative Bragg peak intensity for the (620) Bragg peak in Fig. S1, where we also include the corresponding experimental data points. Several Bragg peaks share the same absolute value $|\mathbf{q}|$ of the scattering vector. Due to the laser excitation, the thickness of the film oscillates and the absolute value $|\mathbf{q}|$ of the scattering vector changes for some of the Bragg peaks. In this way, $|\mathbf{q}|$ of some Bragg peaks moves out

of the measured interval $\big[|\mathbf{G}_{hkl}| - \Delta q, |\mathbf{G}_{hkl}| + \Delta q\big]$, which dramatically influences the measured intensity. We show this, as an example, for the (620) Bragg peak in Fig. S2, where we present the $|\mathbf{q}|$-dependent relative intensity at selected times after the laser-excitation and where we indicate the used interval $\big[|\mathbf{G}_{620}| - \Delta q, |\mathbf{G}_{620}| + \Delta q\big]$ by a gray area.

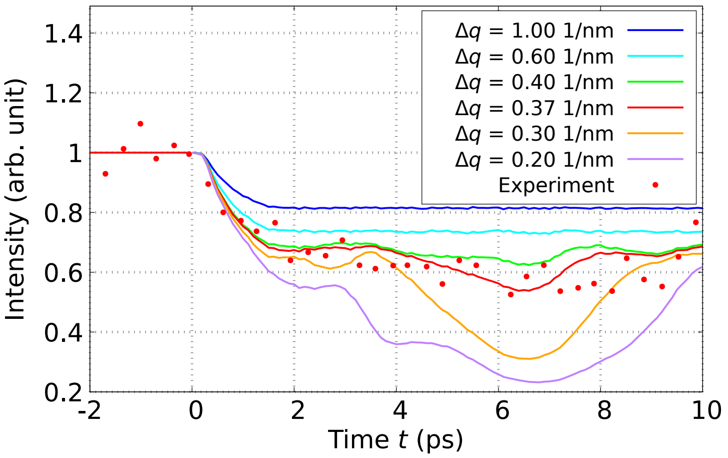


Fig. S1: Time-dependent relative intensity of the (620) Bragg peak is shown for several broadenings $\Delta q$. The points correspond to the measured (620) Bragg peak intensities taken from Figure 4 of Ref. [2].

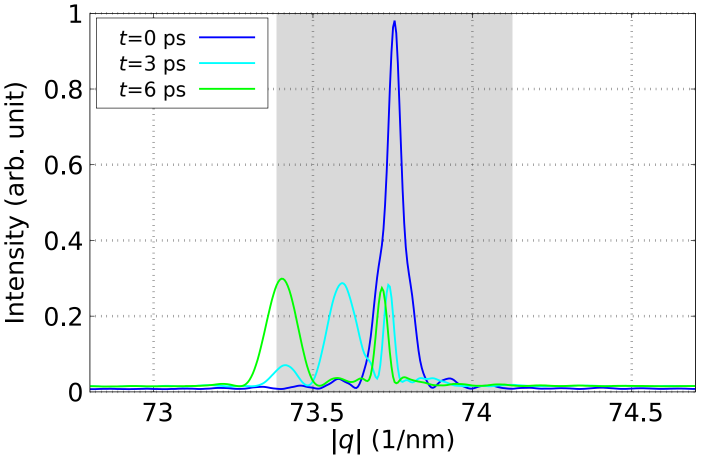


Fig. S2: Realtive scattering intensity is shown as a function of the absolute value $|\mathbf{q}|$ of the scattering vector for values close to $|\mathbf{G}_{620}| = 73.76\,\mathrm{nm}^{-1}$. The gray area indicates the considered interval $\big[|\mathbf{G}_{620}| - \Delta q, |\mathbf{G}_{620}| + \Delta q\big]$ used to compare with the experiment.

In the next step, we analyzed the influences of the excited PES and EPC on the time behavior of the Bragg peak intensities.

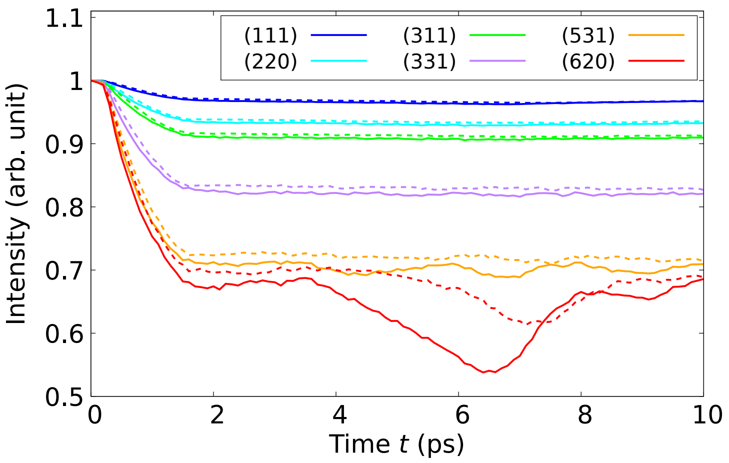


Fig. S3: Relative intensities of various Bragg peaks are shown as a function of time obtained from the MD simulation considering the excited PES & EPC (solid lines) and the MD simulation considering only the EPC (dashed lines).

By comparing the results from the three scenarios of MD simulations – excited PES & EPC, only EPC, only excited PES – we found out that the relative Bragg peak decay is dominated by the EPC whereas the influence of the excited PES is small. In Fig. S3, we present the calculated relative intensities of the Bragg peaks obtained from the MD simulation considering excited PES and EPC and from the MD simulation only considering the EPC. One can clearly see that the relative intensities obtained from the two different MD simulations are almost identical. In addition, the relative intensities keep almost unaffected in the MD simulation which only considers the excited PES (not shown).

Harb *et al.* derived the time-dependent ionic temperature $T_\mathrm{i}$ of the Si film from the time-dependent Bragg peak intensities using Debye Waller theory. In Fig. S4, we show the ionic temperature $T_\mathrm{i}$ as a function of time obtained by Harb *et al.* and obtained from our three different MD simulations.

Fig. S4 clearly shows that the experimentally obtained $T_\mathrm{i}$ is well explained within the error bars by our MD simulation considering the excited PES and the EPC and by our MD simulation only considering the EPC. In Fig. S5, we present the electronic and ionic temperatures as a function of time obtained from our three different scenarios of MD simulations. $T_\mathrm{e}$ is firstly increased due to the laser excitation. Then, $T_\mathrm{e}$ is decreased and $T_\mathrm{i}$ is increased due to

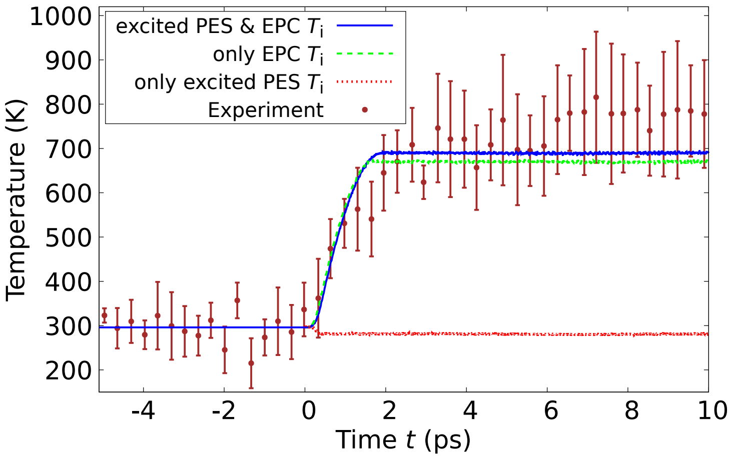


Fig. S4: Ionic temperature $T_i$ is shown as a function of time obtained from the experiment (points with error bars) using Debye Waller theory and from our calculations (lines). The experimental values are taken from Figure 5 of Ref. [2].

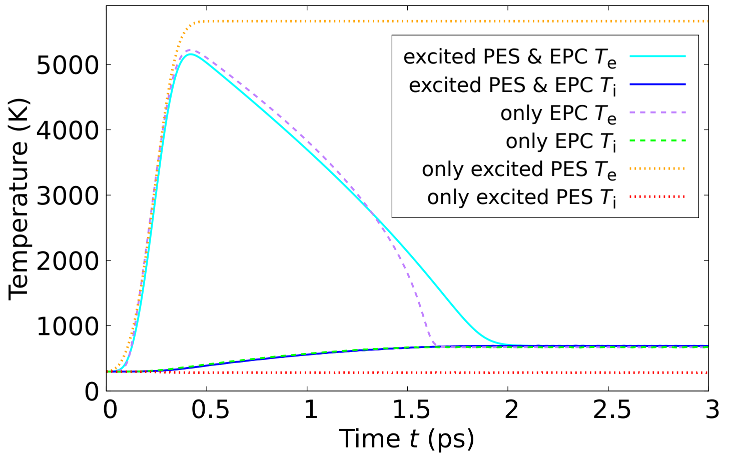


Fig. S5: Electronic and ionic temperatures are show as a function of time obtained from our calculations.

the EPC until both temperatures reach the same value.

## 2.3 Femtosecond-laser excitation above the damage threshold

In a second measurement, Harb *et al.* prepared a free standing monocrystalline Si film with a thickness of $d_{\text{film}} = 30$ nm [3]. They again excited

this film by an intense femtosecond laser-pulse with a central wavelength of $\lambda = 387$ nm and a FWHM-time width of $\tau = 150$ fs. The fluence of $I_{\mathrm{L_{tot}}} = 65\,\frac{\mathrm{mJ}}{\mathrm{cm}^2}$ was absorbed at the surface, which is above the damage threshold. They again measured the time-dependent intensity of the (220) Bragg peak using ultrafast electron diffraction.

To compare directly with this measurement, we set up a simulation cell that consist of $11 \times 11 \times 56$ conventional cells and contains $N_{\mathrm{at}} = 54208$ Si atoms. We applied periodic boundary conditions in $x$- and $y$-direction and applied open boundary conditions in $z$-direction ([$\bar{1}$11] direction of the crystal structure) to get a 30 nm thick Si film. We applied the Andersen thermostat [1] to initialize the atomic coordinates and velocities at $T_{\mathrm{i}} = 300$ K. Then we performed MD simulations of the femtosecond-laser excitation using the three different methods – excited PES & EPC, only excited PES, only EPC. We used a time step of $\Delta t = 1$ fs and simulated a Gaußian-shaped pulse with a FWHM-time width of $\tau = 150$ fs and set for the by the laser absorbed energy $E_{\mathrm{L_{tot}}}$ in the 30 nm thick film

$$\frac{E_{\mathrm{L_{tot}}}}{N_{\mathrm{at}}} = \left(1 - {}^{-\alpha_{\mathrm{abs}}\, d_{\mathrm{film}}}\right) \frac{I_{\mathrm{L_{tot}}}}{d_{\mathrm{film}}\,\rho_{\mathrm{at}}} \approx 1.2\,\frac{\mathrm{eV}}{\mathrm{atom}} \tag{S30}$$

which we obtained from the previously derived absorption coefficient $\alpha_{\mathrm{abs}} = 0.0204569\,\frac{1}{\mathrm{nm}}$, the ab-initio equilibrium atomic density $\rho_{\mathrm{at}} = 50.8414\,\frac{\mathrm{atoms}}{\mathrm{nm}^3}$, and the experimental absorbed laser fluence $I_{\mathrm{L_{tot}}} = 65\,\frac{\mathrm{mJ}}{\mathrm{cm}^2} = 4056.98\,\frac{\mathrm{eV}}{\mathrm{nm}^2}$ at the surface.

We derived the time-dependent intensity of the (220) Bragg peak from the atomic coordinates by considering all Bragg peaks in the interval $\left[|\mathbf{G}_{220}| - \Delta q, |\mathbf{G}_{220}| + \Delta q\right]$, since Harb *et al.* measured the (220) Bragg peak again by averaging over the intensities inside a ring of the measured diffraction image. In Fig. S6, we present our obtained time-dependent intensities for various $\Delta q$ for the MD simulation considering excited PES & EPC together with Harb's results. The value of $\Delta q$ controls mainly the remaining intensity after the Bragg peak is decayed. The remaining intensity increases with increasing $\Delta q$, since one measures more of the background intensity for bigger $\Delta q$. We chose $\Delta q = 0.6\,\frac{1}{\mathrm{nm}}$, since then the rest intensity of the experiment is well reproduced by our calculations.

In Fig. S7, we present the electronic and ionic temperatures as a function of time for our three different scenarios of MD simulations. If the EPC is taken into account, the final ionic temperature is higher, when the excited PES is also taken into account, since the bonds become weaker.

Harb *et al.* also prepared a polycrystalline Si film of $d_{\mathrm{film}} = 50$ nm thickness. They excited also this film by an intense femtosecond laser-pulse with a central wavelength of $\lambda = 387$ nm and a FWHM-time width of $\tau =$

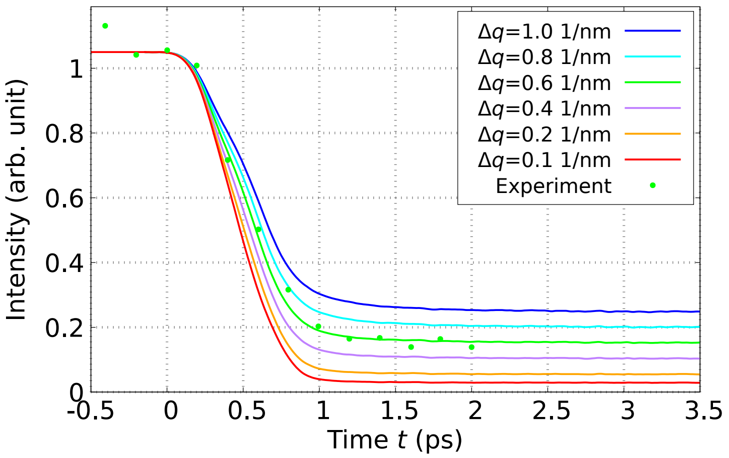


Fig. S6: Time-dependent relative intensity of the (220) Bragg peak is shown for several broadenings $\Delta q$. The points correspond to the measured (220) Bragg peak intensities taken from FIG. 3 (c) of Ref. [3].

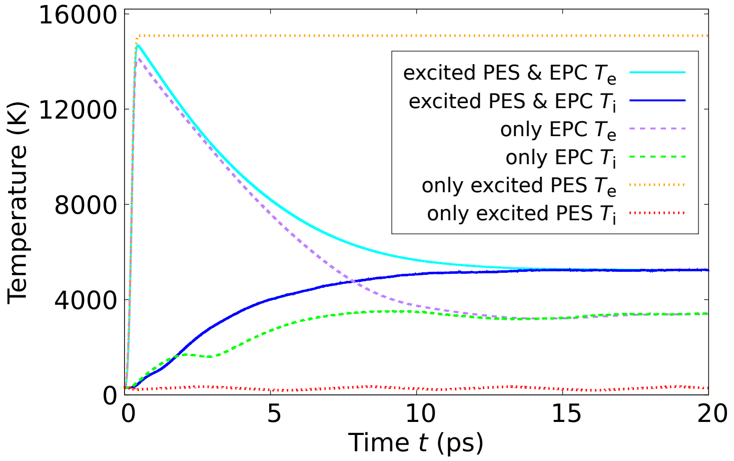


Fig. S7: Electronic and ionic temperatures are show as a function of time for the 30 nm Si film obtained from our calculations.

150 fs, so that the fluence of $I_{\mathrm{L_{tot}}} = 65\,\frac{\mathrm{mJ}}{\mathrm{cm}^2}$ was absorbed at the surface. They measured the time-dependent intensity of serveral Bragg peaks using ultrafast electron diffraction.

In order to compare with this measurement, we utilized the previously generated simulation cell that consists of $11 \times 11 \times 93$ conventional cells and contains $N_{\mathrm{at}} = 90024$ Si atoms. The atoms form a 50 nm thick Si film and were previously thermalized at $T_{\mathrm{i}} = 300$ K. Again, we performed MD simulations of the femtosecond-laser excitation using the three different

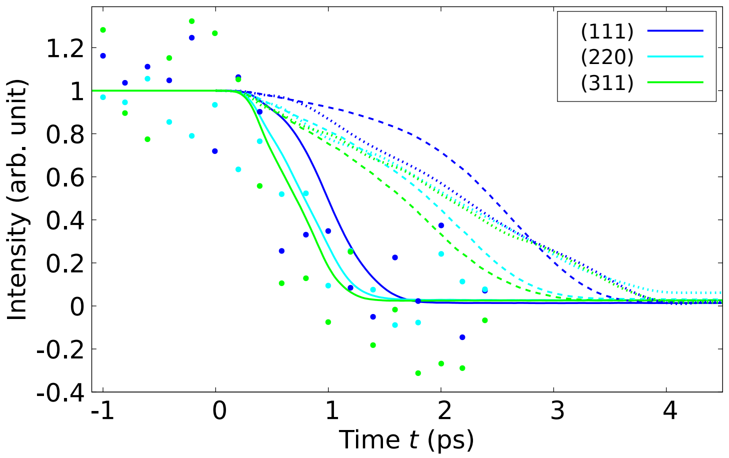


Fig. S8: Relative intensities of several Bragg peaks are shown as a function of time for the 50 nm Si film obtained from the experiment (points) and from the MD simulation considering excited PES & EPC (solid lines), from the MD simulation considering excited PES (dotted lines) and from the MD simulation considering EPC (dashed lines). The experimental values are taken from FIG. 3 (a) of Ref. [3].

scenarios. We simulated a Gaußian-shaped pulse with a FWHM-time width of $\tau = 150$ fs and we set for the energy $E_{\mathrm{L_{tot}}}$ that is absorbed from the laser in the 50 nm thick film

$$\frac{E_{\mathrm{L_{tot}}}}{N_{\mathrm{at}}} = \left(1 - {}^{-\alpha_{\mathrm{abs}}\, d_{\mathrm{film}}}\right) \frac{I_{\mathrm{L_{tot}}}}{d_{\mathrm{film}}\, \rho_{\mathrm{at}}} \approx 1.0\, \frac{\mathrm{eV}}{\mathrm{atom}}. \tag{S31}$$

We derived the time-dependent intensities of the three measured Bragg peaks (111), (220), and (311) from the atomic coordinates and present the obtained results together with the experimental results in Fig. S8. One can clearly see that the experimental data points spread a lot indicating that the measurement may be not so accurate. The inaccuracy is further confirmed by the presence of points with a negative intensity. Harb *et al.* concluded from their measurement that the three Bragg peaks decay with a similar speed. This conclusion may be correct from the available data points of the measurement. However, our calculations show that the (111) Bragg peak decays significantly slower than the two other ones. This agrees with Debye Waller theory, since the (111) Bragg peak belongs to a wave vector with a significant smaller absolute value than the other Bragg peaks. The MD simulation considering only the excited PES and the MD simulation considering only the EPC generate again a to slow Bragg peak decay compared to the experiment. The (111) Bragg peak also decays slower compared to the other

ones for the MD simulation considering only the EPC. For the MD simulation considering only the excited PES, all Bragg peaks decay in a similar way.

# References


[1] Andersen, H. C. *Molecular dynamics simulations at constant pressure and/or temperature.* The Journal of Chemical Physics **72**, 4 (Feb 1980), p. 2384–2393.

[2] Harb, M. and Ernstorfer, R. and Dartigalongue, T. and Hebeisen, C. T. and Jordan, R. E. and Miller, R. J. D. *Carrier relaxation and lattice heating dynamics in silicon revealed by femtosecond electron diffraction.* The Journal of Physical Chemistry B **110**, 50 (Nov 2006), p. 25308–25313. PMID: 17165976.

[3] Harb, M. and Ernstorfer, R. and Hebeisen, C. T. and Sciaini, G. and Peng, W. and Dartigalongue, T. and Eriksson, M. A. and Lagally, M. G. and Kruglik, S. G. and Miller, R. J. D. *Electronically driven structure changes of si captured by femtosecond electron diffraction.* Phys. Rev. Lett. **100** (Apr 2008), p. 155504.

[4] Lide, David R. *Handbook of Chemistry and Physics*, 84th ed. CRC press, 2004.

[5] Swope, W. C. and Andersen, H. C. and Berens, P. H. and Wilson, K. R. *A computer simulation method for the calculation of equilibrium constants for the formation of physical clusters of molecules: Application to small water clusters.* The Journal of Chemical Physics **76**, 1 (1982), p. 637–649.
